# Supplementary material for: Electron spin resonance and spin-valley physics in a silicon double quantum dot
Source: arXiv:1311.5937 source file (2014-08-04)
Supplement: Supplementary file 1 [file supp_ESR_arXiv.pdf]

# SUPPLEMENTARY INFORMATION

## Electron spin resonance and spin-valley physics in a silicon double quantum dot

Xiaojie Hao,[1] Rusko Ruskov,[2] Ming Xiao,[1] Charles Tahan,[2] and HongWen Jiang[1]

[1]*Department of Physics and Astronomy, University of California at Los Angeles, 405 Hilgard Avenue, Los Angeles, California 90095, USA*

[2]*Laboratory for Physical Sciences, 8050 Greenmead Dr., College Park, MD 20740, USA*

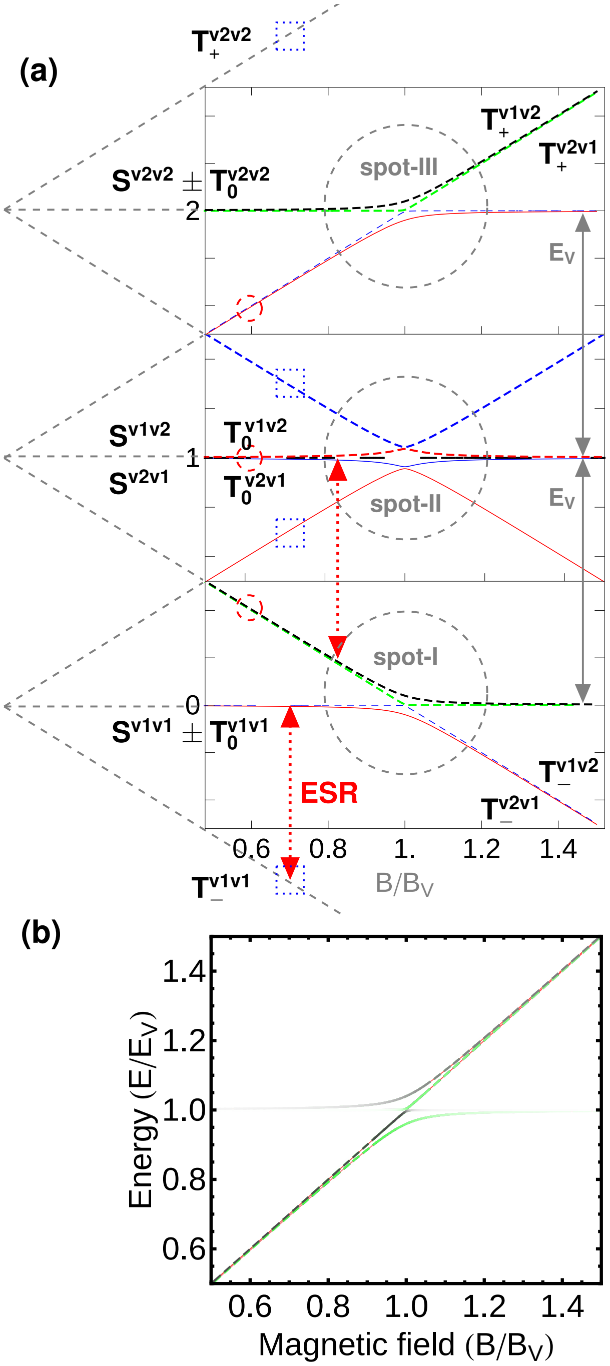


**Supplementary Figure** 1: Level structure and ESR spectroscopy for equal valley splitting, ($\delta \equiv E_V^L - E_V^R = 0$), and zero exchange splitting, $J = 0$. (**a**) The 16 spin-valley states in the $(1,1)$ configuration as a function of magnetic field. The anticrossing spots I,II,III, are defined by only two matrix elements, $a_R$, $b_L$, Eqs. (9), (10); level degeneracy out of anticrossing. The spin-blocked states are shown (dotted rectangles), while the spin-valley blocked states $\mathrm{T}^{v1v2} + \mathrm{T}^{v2v1}$ (dotted circles) are degenerate with some non-blocked states (Supplementary Note 2). The ESR is shown (red dotted arrows), while similar transitions for upper pairs of energy levels are also possible (not shown). (**b**) ($a_R = 0.02$, $b_L = 0.002$ in units of $E_V$ are used for illustration) The ESR signal simulated by combining the energy differences in (**a**) with the AC couplings Eq. (22) reveals one anticrossing of size $\sim |a_R|$, while the second anticrossing, for $b_L \ll a_R$ is almost invisible.

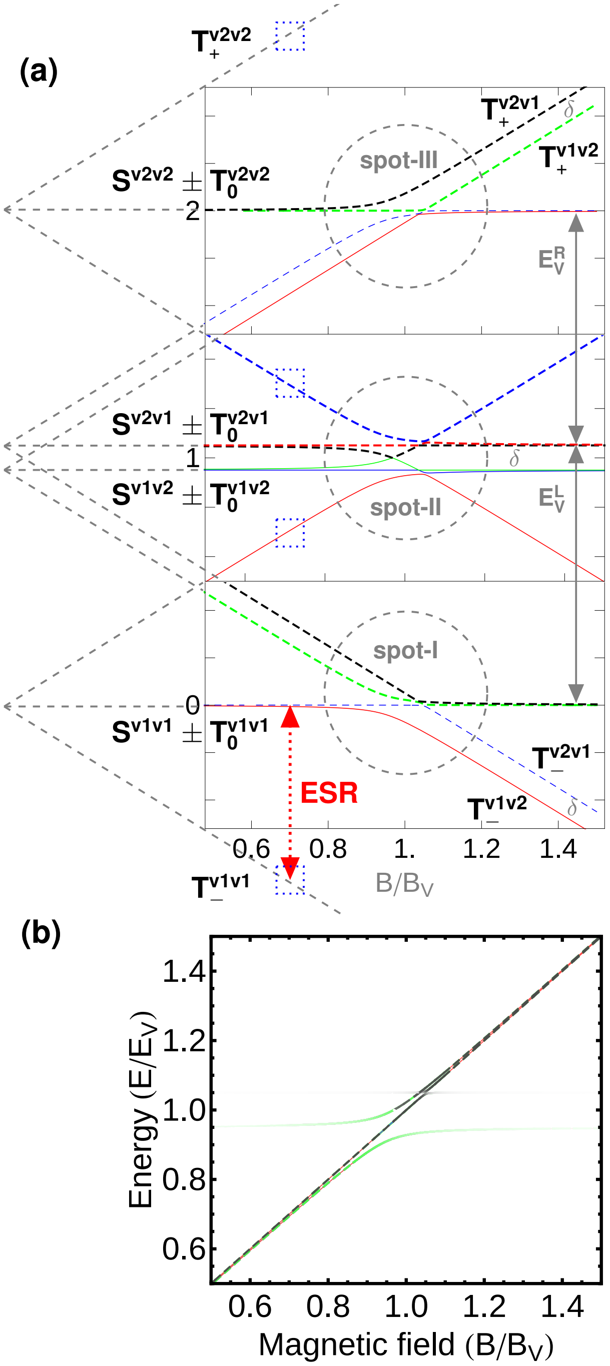


**Supplementary Figure** 2: Level structure and ESR spectroscopy for different valley splitting, $E_V^L > E_V^R$, and zero exchange splitting. (**a**) The 16 spin-valley states in the $(1, 1)$ configuration as a function of magnetic field. The anticrossings are defined by the same dipole matrix elements, $a_R$, $b_L$; level degeneracy out of anticrossing is partially lifted. The spin-blocked states (dotted rectangles) are shown, while there are no spin-valley blocked states, see Supplementary Note 4. (**b**) ($a_R = 0.02$, $b_L = 0.002$, $\delta = 0.1$ in units of $E_V$ are used) While the different valley splitting might provide a multiple anticrossing picture, the ESR signal simulated via the variative AC couplings, Eq. (22), reveals the same anticrossing pattern as for $\delta = 0$, but shifted by $\delta$. This case is unrealistic since the suppression of the ESR signal out of anticrossing cannot be explained, see Supplementary Note 3.

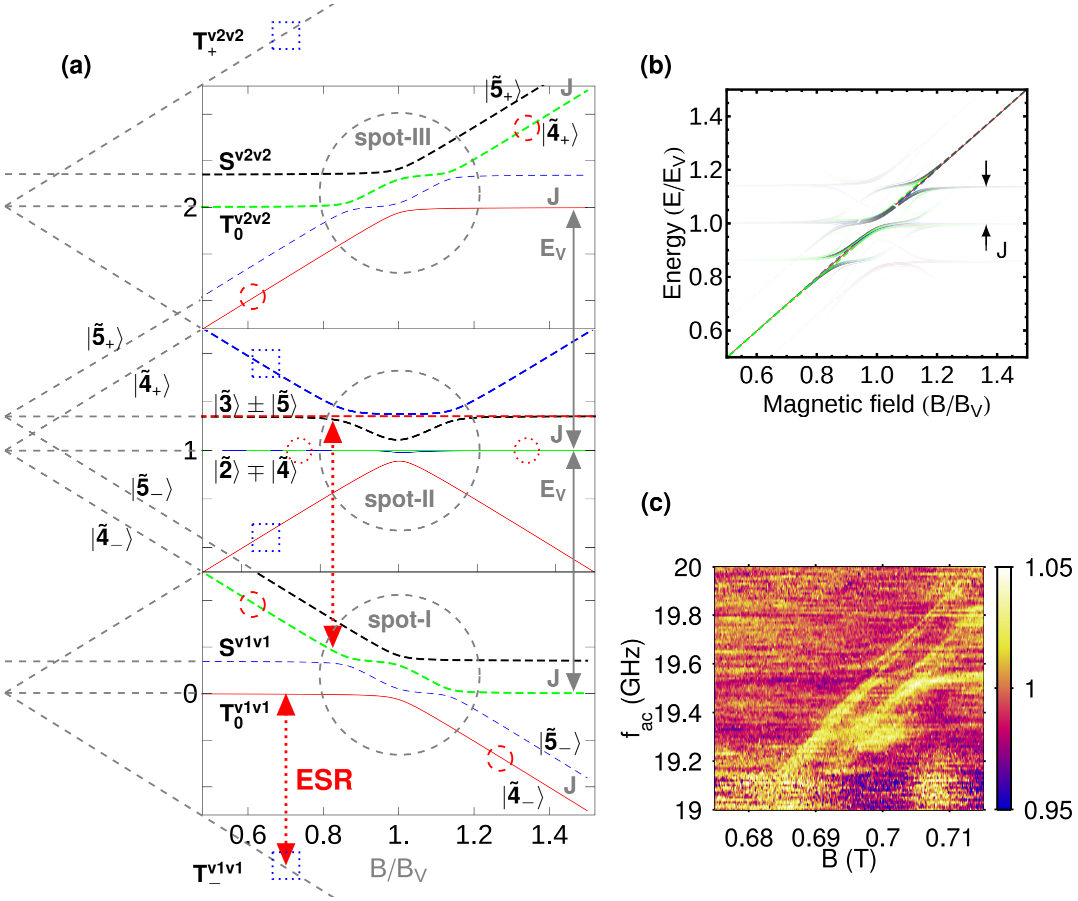


**Supplementary Figure** 3: Level structure and ESR spectroscopy for $J \neq 0$ ($\delta = 0$). (**a**) The 16 spin-valley states in the $(1, 1)$ configuration as a function of magnetic field. Multiple anticrossing picture of energy levels is shown for $J \gg |a_R| \gg |b_L|$ ($J = 0.14$, $a_R = 0.02$, $b_L = 0.002$ are used for illustration.) The structure of anticrossings will change for another regime $|a_R| \gtrsim J \gg |b_L|$, see Fig. 5b of main text. Dotted (blue) rectangles label the spin-blocked states; Dotted (red) circles label the spin-valley blocked states: $|\tilde{4}\rangle = \mathrm{T}_0^{\mathrm{v1v2}} + \mathrm{T}_0^{\mathrm{v2v1}}$, $|\tilde{4}_\pm\rangle = \mathrm{T}_\pm^{\mathrm{v1v2}} + \mathrm{T}_\pm^{\mathrm{v2v1}}$, eventually surviving for a non-ideal interface (see Eqs. (37),(38), and Supplementary Note 4). The other (non-blocked) states are: $|\tilde{5}\rangle = -\mathrm{T}_0^{\mathrm{v1v2}} + \mathrm{T}_0^{\mathrm{v2v1}}$, $|\tilde{5}_\pm\rangle = -\mathrm{T}_\pm^{\mathrm{v1v2}} + \mathrm{T}_\pm^{\mathrm{v2v1}}$, and $|\tilde{2}\rangle = \mathrm{S}^{\mathrm{v1v2}} - \mathrm{S}^{\mathrm{v2v1}}$, $|\tilde{3}\rangle = \mathrm{S}^{\mathrm{v1v2}} + \mathrm{S}^{\mathrm{v2v1}}$ (see text). The spin-blocked or spin-valley blocked states are well separated in energy from the other non-blocked states. (**b**) The non-zero exchange splitting does provide multiple anticrossings, shown by the simulated ESR signal. More accurate description of the ESR signal will require complete study of the related transport rate equation (to be published elsewhere). (**c**) Experimentally measured ESR multiple anticrossing spectroscopy at a different biasing triangle with different cool down.

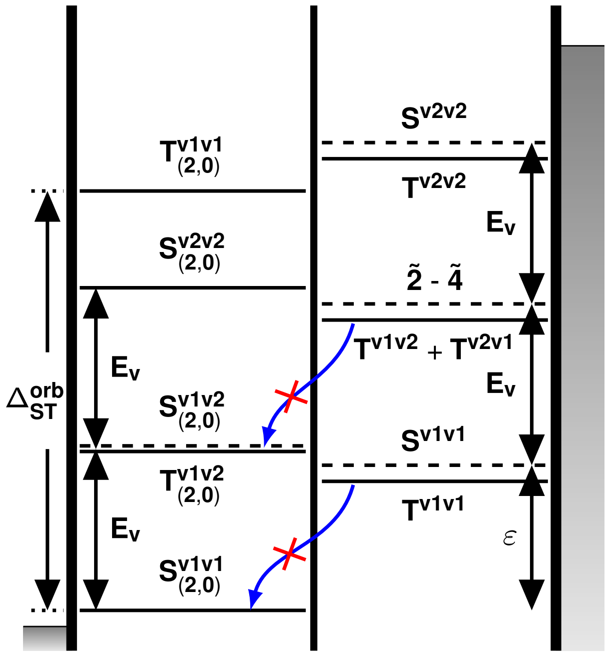


(a)

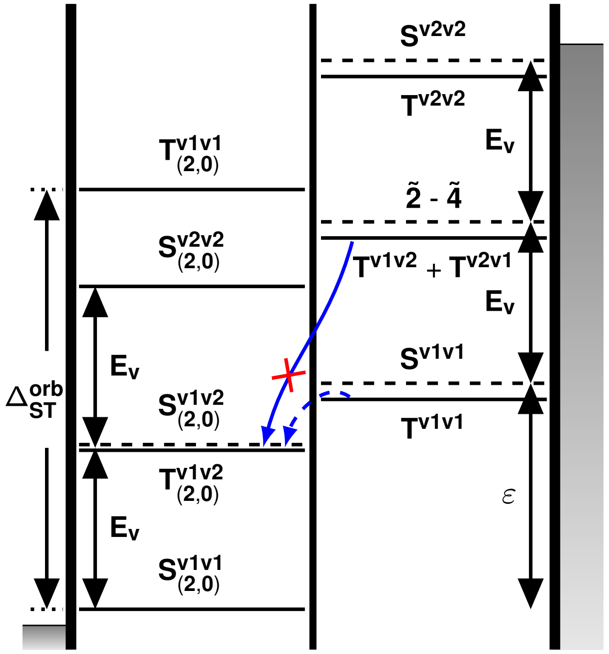


(b)

**Supplementary Figure** 4: Schematic of the spin blockade vs. spin-valley blockade in case of $\Delta_{ST} > 2E_V$. (a) For $\varepsilon < E_V$ the triplet state $T^{\mathrm{v1v1}}$ is spin-blocked, and the state $|\tilde{4}\rangle \sim T^{\mathrm{v1v2}} + T^{\mathrm{v2v1}}$ is spin-valley blocked. (b) For $\varepsilon > E_V$ the spin blockade is lifted due to SOC and a non-ideal interface: $T^{\mathrm{v1v1}} \to T^{\mathrm{v1v2}}_{(2,0)}$. The spin-valley blockade of the state $T^{\mathrm{v1v2}} + T^{\mathrm{v2v1}}$ persists until $\varepsilon \leq \Delta_{ST} - E_V$, where transition to the first orbital excited state is possible: $T^{\mathrm{v1v2}} + T^{\mathrm{v2v1}} \to T^{\mathrm{v1v1}}_{(2,0)}$.

# Supplementary Note 1

## Electron states in quantum dots with valleys

We consider a large double quantum dot (DQD) defined electrostatically in a MOS $Si/SiO_2$ heterostructure, as described in the main text. For a single QD occupied by a single electron an electrostatic energy of $E_C = 2.5\,\mathrm{meV}$ would correspond to the first excited orbital state of some $0.35-0.45\,\mathrm{meV}$ above the ground state and it only weakly influences the ground state shell. Due to strong electric field at the heterostructure, the 6-fold degeneracy of the conduction band electrons is lifted: only two lowest energy valleys remain relevant, at momentums $\boldsymbol{k} \approx k_0\,[\hat{z}, -\hat{z}]$, with $k_0 \simeq 0.85\,\frac{2\pi}{a_0}$; the remaining two-fold degeneracy is lifted via the sharp interface potential, leading to a valley splitting, $E_{\mathrm{V}}$, of the order of few hundred $\mu$eV, and linearly proportional to the electric field at the interface, as experimentally demonstrated recently[1]. This forms the ground state shell of the two lowest valley states, $\mathrm{v}_1, \mathrm{v}_2$.

*Valley wave functions for non-ideal interface.*
In the effective mass approximation the valley wave functions are generally written as

$$|\mathrm{v}_1\rangle = \sum_{\mathrm{i}=\pm\mathrm{z}} \Phi^{\mathrm{i}}_{\mathrm{v}1}(\mathbf{r})\alpha^{\mathrm{v}_1}_{\mathrm{i}}\mathrm{u}_{\mathrm{i}}(\mathbf{r})\,\mathrm{e}^{\mathrm{i}k_{\mathrm{i}}\mathrm{z}} \tag{1}$$

$$|\mathrm{v}_2\rangle = \sum_{\mathrm{i}=\pm\mathrm{z}} \Phi^{\mathrm{i}}_{\mathrm{v}2}(\mathbf{r})\alpha^{\mathrm{v}_2}_{\mathrm{i}}\mathrm{u}_{\mathrm{i}}(\mathbf{r})\,\mathrm{e}^{\mathrm{i}k_{\mathrm{i}}\mathrm{z}}, \tag{2}$$

where $\psi_i(\mathbf{r}) \equiv u_i(\mathbf{r})\,e^{ik_iz}$ are the Kohn-Luttinger valley functions, with the periodic part $u_i(\mathbf{r})$, and $k_i$ $(i = \pm z)$ is the position of the valley minima. Here, $\Phi^{i}_{\mathrm{v_j}}(\mathbf{r})$ are the envelope functions corresponding to the orbital ground state ($s$-like). In the ideal QD (ideal interface, symmetric circular dot, etc.) the envelopes are separable, e.g.: $\Phi^{+z}_0(\mathbf{r}) = F_0(x,y)\,f_0(z)$. Generally, the index of the state, $\mathrm{v}_1$ or $\mathrm{v}_2$, distinguishes different envelopes, originating from valley-orbit coupling in the presence of a non-ideal interface; also separability may be lost. The relations: $\Phi^{+z}_{\mathrm{v_j}} = \Phi^{-z}_{\mathrm{v_j}}$ and $|\alpha^{\mathrm{v_j}}_{+z}| = |\alpha^{\mathrm{v_j}}_{-z}|$ are maintained for each state by time reversal. Assuming relatively strong electric field at the interface (and therefore states of definite parity[2]), the valley populations are: $\alpha^{\mathrm{v}_1}_{+z} = -\alpha^{\mathrm{v}_1}_{-z} = \frac{1}{\sqrt{2}}$, $\alpha^{\mathrm{v}_2}_{+z} = \alpha^{\mathrm{v}_2}_{-z} = \frac{1}{\sqrt{2}}$.

*Defining the 16 states of the* $(1,1)$ *configuration.*
To introduce the two-electron delocalized states $(1,1)$ we use the orthogonalized single electron states for the left and right dots, $\tilde{L}(\mathbf{r})$, $\tilde{R}(\mathbf{r})$. Here L and R are reserved for the lowest energy ($s$-like) states with the overlap integral $\mathcal{L} \equiv \langle L|R\rangle \sim e^{-\frac{d^2}{a_D^2}} \ll 1$. ($2d$ is the distance between the dots and $a_D$ is the dot radius). Their orthogonalized counterparts $\tilde{L} \approx L$, $\tilde{R} \approx R$ obey the condition $\langle\tilde{L}|\tilde{R}\rangle = 0$, and are defined as[3,4]

$$\tilde{L} = \frac{L - g_aR}{\sqrt{1-2\mathcal{L}g_a + g_a^2}}, \quad \tilde{R} = \frac{R - g_aL}{\sqrt{1-2\mathcal{L}g_a + g_a^2}}, \tag{3}$$

with the admixture factor $g_a \equiv (1-\sqrt{1-\mathcal{L}^2})/\mathcal{L} \ll 1$. For further reference, we also introduce the notation of higher orbital single-electron states in each dot, $\tilde{Q}_{\mathrm{L,R}}(x)$, which are well separated in energy from the ground state shell, and their influence on the lowest electron states is supposed to be small.

In Si all these states acquire an additional valley index $\mathrm{v_i}$, $\mathrm{i} = 1,2$, so that, e.g., $\tilde{R}_{\mathrm{v_i}}(\mathbf{r})$ is the ground states wave function of a single electron in the right dot in the valley $\mathrm{v_i}$, etc., with the valley splitting $E^R_V \equiv E^R_{\mathrm{v}2} - E^R_{\mathrm{v}1}$. We also reserve the possibility of different valley splitting in each dot: $E^R_V \neq E^L_V$, in general.

With the above definitions the 16 lowest states of the $(1,1)$-charge configuration are built in the Hund-Milliken approximation[4], e.g., for the lowest valley configuration $[\mathrm{v}_1, \mathrm{v}_1]$ one gets a singlet and a triplet

$$S^{\mathrm{v1v1}}(\mathbf{r}_1,\mathbf{r}_2) \equiv |S\rangle \times\frac{1}{\sqrt{2}}\left(\tilde{L}_{\mathrm{v}_1}(\mathbf{r}_1)\tilde{R}_{\mathrm{v}_1}(\mathbf{r}_2) + \tilde{L}_{\mathrm{v}_1}(\mathbf{r}_2)\tilde{R}_{\mathrm{v}_1}(\mathbf{r}_1)\right) \tag{4}$$

$$T^{\mathrm{v1v1}}(\mathbf{r}_1,\mathbf{r}_2) \equiv |T_{\pm,0}\rangle \times\frac{1}{\sqrt{2}}\left(\tilde{L}_{\mathrm{v}_1}(\mathbf{r}_1)\tilde{R}_{\mathrm{v}_1}(\mathbf{r}_2) - \tilde{L}_{\mathrm{v}_1}(\mathbf{r}_2)\tilde{R}_{\mathrm{v}_1}(\mathbf{r}_1)\right), \tag{5}$$

where $|S\rangle \equiv \frac{1}{\sqrt{2}}[|\Uparrow_1\Downarrow_2\rangle - |\Uparrow_2\Downarrow_1\rangle]$, $|T_+\rangle \equiv |\Uparrow_1\Uparrow_2\rangle$, $|T_-\rangle \equiv |\Downarrow_1\Downarrow_2\rangle$, and $|T_0\rangle \equiv \frac{1}{\sqrt{2}}[|\Uparrow_1\Downarrow_2\rangle + |\Uparrow_2\Downarrow_1\rangle]$ are the two-electron spin states. The states with mixed valley content $[\mathrm{v}_1, \mathrm{v}_2]$ are of two kinds, depending on which valley is occupied in each dot. E.g., there are two singlet states $S^{\mathrm{v1v2}}(\mathbf{r}_1,\mathbf{r}_2)$, $S^{\mathrm{v2v1}}(\mathbf{r}_1,\mathbf{r}_2)$, and two triplets $T^{\mathrm{v1v2}}(\mathbf{r}_1,\mathbf{r}_2)$, $T^{\mathrm{v2v1}}(\mathbf{r}_1,\mathbf{r}_2)$, where

the valley indices in Eqs. (4), (5), should be replaced accordingly (i.e., $(\mathrm{v}_1, \mathrm{v}_1) \to (\mathrm{v}_1, \mathrm{v}_2)$ or $(\mathrm{v}_1, \mathrm{v}_1) \to (\mathrm{v}_2, \mathrm{v}_1)$). In the absence of magnetic field these 8 states are degenerate and split off from the $[\mathrm{v}_1, \mathrm{v}_1]$ states by $E_V^R$ ($E_V^L$). Finally, the upper valley states $[\mathrm{v}_2, \mathrm{v}_2]$ are again a singlet and a triplet, similar to Eqs. (4), (5), with the replacement $(\mathrm{v}_1, \mathrm{v}_1) \to (\mathrm{v}_2, \mathrm{v}_2)$, and energy $E_V^R + E_V^L \equiv 2E_V$.

# Supplementary Note 2
## Spin-valley mixing

*The valley mixing dipole matrix elements.*
Under switching on an external magnetic field the degeneracy of the $(1,1)$-levels is partially lifted: the polarized triplets get a Zeeman energy shift of $E_Z = \pm g\mu_B B$, so that at $|E_Z| \approx E_V$ they will cross the corresponding unpolarized states of a different valley content. E.g., the triplets $T_-^{\mathrm{v1v2}}$ and $T_-^{\mathrm{v2v1}}$ (anti) cross with the lowest unpolarized states, $S^{\mathrm{v1v1}}$ and $T_0^{\mathrm{v1v1}}$ at $E \approx 0$, forming the (anti) crossing Spot I of 4 levels (see Supplementary Figure 1a). Similarly, the triplets $T_+^{\mathrm{v1v2}}$ and $T_+^{\mathrm{v2v1}}$ cross the unpolarized states, $S^{\mathrm{v2v2}}$ and $T_0^{\mathrm{v2v2}}$ at $E \approx 2E_V$, forming the (anti) crossing Spot III (see Supplementary Figure 1a). Finally, the (anti) crossing Spot II (see Supplementary Figure 1a), at energy $E \approx E_V$, is due to 6 states: the two triplet states $T_+^{\mathrm{v1v1}}$ and $T_-^{\mathrm{v2v2}}$ will cross the unpolarized states of a mixed valley content, namely $S^{\mathrm{v1v2}}$, $S^{\mathrm{v2v1}}$, $T_0^{\mathrm{v1v2}}$, and $T_0^{\mathrm{v2v1}}$. Here, Supplementary Figure 1, for simplicity we have neglected the finite exchange energy $J$, which physically corresponds to the situation $J \ll E_N$ when the nuclear hyperfine (HF) mixing is dominating. Later we will argue that in this regime the experimentally observed characteristic behavior of the ESR signal cannot be explained, see Supplementary Note 3.

Considering possible mixing of these states, notice that a spin-orbit coupling (SOC) at the Si/$SiO_2$-interface can flip a single spin, for an ideal interface, but it cannot mix different valleys and one would observe a true crossing. However, the SOC interaction can mix states of different valley content for a non-ideal interface[1].

The anticipated non-zero splitting will require non-zero dipole matrix elements, e.g.,

$$\mathbf{r}_{12}^{R} \equiv \langle \tilde{R}_{\mathrm{v}_1}(1)|\mathbf{r}|\tilde{R}_{\mathrm{v}_2}(1)\rangle \tag{6}$$
$$\mathbf{r}_{12}^{L} \equiv \langle \tilde{L}_{\mathrm{v}_1}(1)|\mathbf{r}|\tilde{L}_{\mathrm{v}_2}(1)\rangle \tag{7}$$

(here and below we use the shorthand notation, $\tilde{L}_{\mathrm{v}_1}(1) \equiv \tilde{L}_{\mathrm{v}_1}(\mathbf{r}_1)$, etc.). These matrix elements are exactly zero for an ideal interface, if one takes into account only intravalley transitions (a non-zero contribution due to an Umklapp process is highly suppressed for the energy scale, $\sim 20\,\mathrm{GHz}$, of interest). Qualitatively, for a non-ideal interface, the envelope function of each of the $s$-like (ground, symmetric) states acquire a (valley dependent) asymmetric contribution ($p$-like, or higher), that leads to a non-zero dipole matrix elements of this type[1,5,6]. Such dipole matrix elements have been introduced recently[1] on a purely phenomenological ground, that have explained successfully the experimentally measured $T_1$-times in a single QD (with 1, 2, 3 electrons), with their magnetic field $B^5 - B^7$-dependence, and including also the so called relaxation hot spots[1]. Recently, similar matrix elements were calculated within a tight-binding approach assuming single atomic steps/roughness within the QD, which leads to the same order of magnitude dipole size[5].

*Spin-orbit 2D coupling and effective Hamiltonians.*
We calculate the splitting at anticrossing of the spin-valley states via the spin-orbit coupling (SOC). In two dimensions the SOC Hamiltonian, $H_{SO} = H_D + H_R$, includes the Dresselhaus and Rashba terms, related to conduction band electrons, confined in a [001] 2DEG:

$$H_D = \beta_D(-\sigma_x\, P_x + \sigma_y\, P_y), \quad H_R = \alpha_R(\sigma_x\, P_y + \sigma_y\, P_x), \tag{8}$$

where $\sigma_x$, $\sigma_y$ are the Pauli matrices along the principal crystal axes, and $\mathbf{P} = \mathbf{p} + e\mathbf{A}(\mathbf{r})$ is the generalized momentum. Related to current experiment, we consider an in-plane magnetic field, which is parallel to the (110)-direction (see Fig. 1a,b of main text), and its vector potential in the symmetric gauge reads: $\mathbf{A}(\mathbf{r}) = \frac{B}{2\sqrt{2}}(z, -z, -x+y)$. Using the eigenoperators $\sigma_{\pm 45} \equiv -(\sigma_x \pm \sigma_y)$, $(\sigma_{+45}|\uparrow,\downarrow\rangle = (\pm)|\uparrow,\downarrow\rangle)$, and Hamiltonian commutation relations one can express the mixing Hamiltonians via the dipole matrix elements:

$$\langle S^{\mathrm{v1v1}}|H_{\mathrm{SO}}|T_-^{\mathrm{v1v2}}\rangle = \frac{i\, m_t\, E_V^R\,(\beta_D - \alpha_R)}{2\hbar}(x_{12}^R + y_{12}^R) \equiv i\, a_R, \tag{9}$$

$$\langle S^{\mathrm{v1v1}}|H_{\mathrm{SO}}|T_-^{\mathrm{v2v1}}\rangle = \frac{-i\, m_t\, E_V^L\,(\beta_D - \alpha_R)}{2\hbar}(x_{12}^L + y_{12}^L) \equiv -i\, b_L, \tag{10}$$

where $x(y)_{12}^{R,L}$ is the $x(y)$ component of $\mathbf{r}_{12}^{R,L}$ in Eq. (6), (7). Notice, that we consider spin-valley mixing matrix elements only between the states involved in the above introduced anticrossing spots, I, II, III, while neglecting matrix elements between states that are well separated in energy (a full Hamiltonian will be given elsewhere).

It is remarkable that all the three mixing Hamiltonians are defined via the same dipole matrix elements, Eqs. (6), (7), combined in the quantities $a_R$, $b_L$, Eqs. (9), (10). Using the basis states $1 \equiv S^{\mathrm{v1v1}}$, $2 \equiv T_0^{\mathrm{v1v1}}$, $3 \equiv T_-^{\mathrm{v1v2}}$, and $4 \equiv T_-^{\mathrm{v2v1}}$, for $H^{\mathrm{I}}$ we get after straightforward calculations:

$$H^{\mathrm{I}} = \begin{pmatrix} 0 & 0 & i\,a_R & -i\,b_L \\ 0 & 0 & -i\,a_R & -i\,b_L \\ -i\,a_R & i\,a_R & X-\delta/2 & 0 \\ i\,b_L & i\,b_L & 0 & X+\delta/2 \end{pmatrix}, \tag{11}$$

where $X \equiv E_V - E_Z$ is the Zeeman energy detuning from the valley splitting energy $E_V \equiv (E_V^L + E_V^R)/2$, and $\delta \equiv E_V^L - E_V^R$ is the possible difference of valley energies in the left and right dot (due to, e.g., a different applied electric field at the dot interface, see, e.g. Ref. 1). Using the basis states of spot II, $T_+^{\mathrm{v1v1}}$, $S^{\mathrm{v1v2}}$, $S^{\mathrm{v2v1}}$, $T_0^{\mathrm{v1v2}}$, $T_0^{\mathrm{v2v1}}$, $T_-^{\mathrm{v2v2}}$, the mixing Hamiltonian is:

$$H^{\mathrm{II}} = \begin{pmatrix} -X & -i\,a_R & i\,b_L & -i\,a_R & -i\,b_L & 0 \\ i\,a_R & -\delta/2 & 0 & 0 & 0 & -i\,b_L \\ -i\,b_L & 0 & \delta/2 & 0 & 0 & i\,a_R \\ i\,a_R & 0 & 0 & -\delta/2 & 0 & -i\,b_L \\ i\,b_L & 0 & 0 & 0 & \delta/2 & -i\,a_R \\ 0 & i\,b_L & -i\,a_R & i\,b_L & i\,a_R & X \end{pmatrix} + E_V. \tag{12}$$

Finally, for the basis states of spot III, $S^{\mathrm{v2v2}}$, $T_0^{\mathrm{v2v2}}$, $T_+^{\mathrm{v1v2}}$, $T_+^{\mathrm{v2v1}}$, for the mixing Hamiltonian one gets:

$$H^{\mathrm{III}} = \begin{pmatrix} 0 & 0 & -i\,b_L & i\,a_R \\ 0 & 0 & i\,b_L & i\,a_R \\ i\,b_L & -i\,b_L & -X-\delta/2 & 0 \\ -i\,a_R & -i\,a_R & 0 & -X+\delta/2 \end{pmatrix} + 2\,E_V. \tag{13}$$

For $\delta \neq 0$ the eigenstates can be calculated analytically using Eqs. (11)-(13). For the spot I we get:

$$E_{1,4} = \frac{1}{2}\left(X - \frac{\delta}{2} \mp f_-(a_R, X, \delta)\right),$$
$$E_{2,3} = \frac{1}{2}\left(X + \frac{\delta}{2} \mp f_+(b_L, X, \delta)\right), \tag{14}$$

where $f_\pm(y, X, \delta) \equiv \sqrt{(X \pm \frac{\delta}{2})^2 + 8y^2}$, and the energies are in increasing order (for $|a_R| > |b_L|$ and $\delta = 0$). For $X > 0$ (Zeeman energy below the valley splitting $E_V$) the unpolarized states are $1, 2$, and the polarized one are $3, 4$. For the spot II, the degeneracy of the 4 unpolarized states is lifted. The eigenstates are symmetric with respect to the energy level $E = E_V$ (Supplementary Figure 2):

$$E_{01} = -E_{02} = \frac{\delta}{2} \tag{15}$$
$$E_{p1} = -E_{m1} = \frac{f_-(a_R, X, \delta) - f_+(b_L, X, \delta)}{4} \tag{16}$$
$$E_{p2} = -E_{m2} = \frac{f_-(a_R, X, \delta) + f_+(b_L, X, \delta)}{4} \tag{17}$$

and for the spot III we obtain, relative to the energy level $E = 2E_V$:

$$E_{1',4'} = -\frac{1}{2}\left(X - \frac{\delta}{2} \pm f_-(a_R, X, \delta)\right) \tag{18}$$
$$E_{2',3'} = -\frac{1}{2}\left(X + \frac{\delta}{2} \pm f_+(b_L, X, \delta)\right) \tag{19}$$

where now the polarized states $1', 2'$ are lower in energy, and the unpolarized one are $3', 4'$. The energy levels for $\delta \neq 0$ are plotted on Supplementary Figure 2a.

To calculate splitting at anticrossing it is instructive to consider first the simplest case, $\delta = 0$ (see Fig. 5 a,c of main text and Supplementary Figure 1). For the spot I the two doubly degenerate levels (the unpolarized one, $1, 2$, and the polarized one, $3, 4$) split and anticross at $E_Z \approx E_V$. In the case when $|a_R| \gg |b_L|$ the anticrossing splitting of $\sim |b_L|$ is negligible, and the energy levels $E_2(E_Z < E_V)$ and $E_3(E_Z > E_V)$ constitute (approximately) a straight horizontal line at $E = 0$. In its turn, the energy levels $E_1$, $E_4$ split at anticrossing by:

$$\Delta_{\mathrm{anti-cross}} = (E_4 - E_1)_{|X=0} = 2\sqrt{2}|a_R|. \tag{20}$$

From Eq. (9), assuming SOC strength of $\beta_D - \alpha_R \approx 15 - 45\,\mathrm{m/s}$ for an interface field of $\sim 10^7\,\mathrm{V/m}$, a transverse mass $m_t \simeq 0.198 m_e$, and the measured $E_V \simeq 86.2\,\mu\mathrm{eV}$, one gets $\Delta_{\mathrm{anti-cross}} \approx 50 - 60\,\mathrm{MHz}$ for a dipole size $r \equiv x_{12}^R = 15 - 55\,\mathrm{nm}$. consistent with the dipole size extracted in the recent $T_1$-relaxation-hot-spot experiment[1]. (We notice that in the experiment[1] the QD has a smaller size, corresponding to orbital splitting $\Delta_{ST} = 8\,\mathrm{meV}$, while in the current experiment the dots are larger: $\Delta_{ST} = 0.35\,\mathrm{meV}$, and so the dipole size of interest). We show below that the same anticrossing splitting will reveal itself in the ESR spectrum, despite the apparently complicated structure of levels, that follow from the three "spot" Hamiltonians, Eqs. (11)-(13). To illustrate qualitatively the "reconstruction" of the ESR spectrum, we consider the simplest case of $\delta = 0$, then elaborate on the effect of different valley splitting. Then we argued on the effect of a finite exchange splitting as well.

# Supplementary Note 3
## Reconstruction of the ESR

*ESR signal and AC coupling.*
The non-zero ESR signal means that a $(1,1)$-state, which is initially spin-blocked (or blocked in another way, see below), can be coupled resonantly to another eigenstate of the $(1,1)$-subsystem, that can subsequently decay inelastically to a $(2,0)$-state, so lifting the blockade. Consider, for example the spin-blocked states $T_{\mp}^{\mathrm{v1v1}}$, which are a direct analog of the spin-blockade in a GaAs DQD system[7]. To lift the blockade a resonant AC microwave field is applied (it is perpendicular to the interface, Fig. 1b of main text), which is expressed with the Hamiltonian

$$\hat{H}_{\mathrm{ac}} = \frac{g\mu_B B_{\mathrm{ac}}}{\sqrt{2}} \cos\omega t \times \left[-i|\mathrm{T}_+\rangle\langle \mathrm{T}_0| + i|\mathrm{T}_-\rangle\langle \mathrm{T}_0| + \mathrm{h.c.}\right] \otimes \mathrm{I}^{\mathrm{v_i v_j}} . \tag{21}$$

Here the unity $\mathrm{I}^{\mathrm{v_i v_j}}$ means that only states with the same valley content are coupled. For two eigenstates (Supplementary Figure 1) as $|i\rangle$, $|j\rangle$, a non-zero signal requires a non-zero AC coupling coefficient:

$$B_{\mathrm{AC}}^{(ij)} = \langle i| \left[-i|\mathrm{T}_+\rangle\langle \mathrm{T}_0| + i|\mathrm{T}_-\rangle\langle \mathrm{T}_0| + \mathrm{h.c.}\right] |j\rangle. \tag{22}$$

As an example, the couplings of the blocked state $0 \equiv T_{-}^{\mathrm{v1v1}}$ to the states that anticross at spot I (for $\delta = 0$) are:

$$B_{AC}^{(01)} = \frac{i\sqrt{f(a_R, X) + X}}{2\sqrt{f(a_R, X)}} \tag{23}$$

$$B_{AC}^{(02)} = \frac{i\sqrt{f(b_L, X) + X}}{2\sqrt{f(b_L, X)}} \tag{24}$$

$$B_{AC}^{(03)} = \frac{-i\sqrt{f(b_L, X) - X}}{2\sqrt{f(b_L, X)}} \tag{25}$$

$$B_{AC}^{(04)} = \frac{-i\sqrt{f(a_R, X) - X}}{2\sqrt{f(a_R, X)}}, \tag{26}$$

with $f(y, X) \equiv f_+(y, X, \delta = 0)$, reflecting the presence of the state $T_0^{\mathrm{v1v1}}$ in each of them. Since the presence of $T_0^{\mathrm{v1v1}}$ varies with the Zeeman splitting in each of the eigenstates, the AC coupling strength and the ESR signal will vary, as well.

In addition to Eqs. (23)-(26), we have calculated all relevant AC couplings between the four levels of spot I and the eigenstates of the spot II Hamiltonian, that are capable to reproduce an energy difference of the order of $\sim E_V$ at $X \sim 0$, and the corresponding energy differences. The energy differences between the four levels of spot III and relevant eigenlevels of spot II were considered as well, together with the corresponding AC couplings, as a function of the Zeeman detuning $X \equiv E_V - E_Z$. Despite the apparently complicated set of energy differences, the AC coupling dependence on $X$ maps out a combined "ESR signal", that consist of just one anticrossing and a straight sloped line in between, see Supplementary Figure 1b. Notice, that for $\delta \neq 0$, analogous calculations brings essentially the same "pattern", just shifted by $\delta$, Supplementary Figure 2b.

While the resulting ESR "reconstruction" captures the decrease of the horizontal ESR line out of anticrossing, the signal decreasing along the sloped line is not reproduced here. This can be improved by noting that, e.g., for $E_Z \ll E_V$, the state $\mathrm{T}_{-}^{\mathrm{v1v1}}$ is *equally AC coupled* to two degenerate states $\pm\mathrm{S}^{\mathrm{v1v1}} + \mathrm{T}_0^{\mathrm{v1v1}}$ (Supplementary Figure 1a, 2a), and in the resulting AC evolution via Eq. (21) the non-blocked state $\mathrm{S}^{\mathrm{v1v1}}$ is exactly canceled. Since the degeneracy of the levels, however, an S-$\mathrm{T}_0$ mixing due to the nuclear hyperfine field (HF) is not suppressed, see Eq. (48). Furthermore, the estimated AC amplitude $B_{\mathrm{ac}} \approx 0.020\,\mathrm{mT}$ is of the order of the HF field $\sigma_N^{\mathrm{Si}}$, and no overdriving suppression is expected either, see, e.g. Ref. 8. The actual suppression can be explained via finite exchange splitting, considered later below.

*ESR signal and selection rules.*
The ESR signal will further depend on the content of the eigenstates that are brought in resonance with a blocked state. Namely, are there any singlets (or some triplet states) that can decay to the corresponding $(2,0)$-states, and thus they would be not blocked? The $(2,0)$-states are the two-electron states in a single (e.g., the left) dot in the case when singlet-triplet (orbital) splitting is much larger than the valley splitting in the dot. We introduce the lowest in

energy singlets:

$$S^{\rm v1v1}_{(2,0)} = \tilde{L}_{\rm v_1}(1)\tilde{L}_{\rm v_1}(2)|S\rangle \tag{27}$$

$$S^{\rm v1v2}_{(2,0)} = \frac{1}{\sqrt{2}}(\tilde{L}_{\rm v_1}(1)\tilde{L}_{\rm v_2}(2) + \tilde{L}_{\rm v_1}(2)\tilde{L}_{\rm v_2}(1))|S\rangle \tag{28}$$

$$S^{\rm v2v2}_{(2,0)} = \tilde{L}_{\rm v_2}(1)\tilde{L}_{\rm v_2}(2)|S\rangle, \tag{29}$$

and the triplet states:

$$T^{\rm v1v2}_{(2,0)} = \frac{1}{\sqrt{2}}(\tilde{L}_{\rm v_1}(1)\tilde{L}_{\rm v_2}(2) - \tilde{L}_{\rm v_1}(2)\tilde{L}_{\rm v_2}(1))|T\rangle. \tag{30}$$

Similar to Ref. 1 we assume that the main mechanism of inelastic tunneling, $|i\rangle_{(1,1)} \to |f\rangle_{(2,0)}$, is due to phonon emission which for Si is due to the deformation potential electron-phonon interaction $\mathcal{H}_{\rm e-ph}$[9]. Assuming that the relevant transitions are energetically allowed, straightforward calculation gives the following Table of phonon decay amplitudes, $\langle f|\mathcal{H}_{\rm e-ph}|i\rangle$, for the singlets:

$$S^{\rm v1v1} \xrightarrow{\sqrt{2}a^{(11)}_{\rm LR}} S^{\rm v1v1}_{(2,0)},\ a^{(11)}_{\rm LR} \equiv \langle \tilde{L}_{\rm v_1}(1)|\mathcal{H}^{(1)}_{\rm e-ph}|\tilde{R}_{\rm v_1}(1)\rangle \tag{31}$$

$$S^{\rm v1v2} \xrightarrow{\sqrt{2}a^{(12)}_{\rm LR}} S^{\rm v1v1}_{(2,0)},\ a^{(12)}_{\rm LR} \equiv \langle \tilde{L}_{\rm v_1}(1)|\mathcal{H}^{(1)}_{\rm e-ph}|\tilde{R}_{\rm v_2}(1)\rangle \tag{32}$$

$$S^{\rm v2v1} \xrightarrow{0} S^{\rm v1v1}_{(2,0)} \tag{33}$$

$$S^{\rm v1v2} \xrightarrow{a^{(22)}_{\rm LR}} S^{\rm v1v2}_{(2,0)},\ a^{(22)}_{\rm LR} \equiv \langle \tilde{L}_{\rm v_2}(1)|\mathcal{H}^{(1)}_{\rm e-ph}|\tilde{R}_{\rm v_2}(1)\rangle \tag{34}$$

$$S^{\rm v2v1} \xrightarrow{a^{(11)}_{\rm LR}} S^{\rm v1v2}_{(2,0)} \tag{35}$$

and an analogous Table of transition amplitudes for the triplets:

$$T^{\rm v1v1} \xrightarrow{a^{(21)}_{\rm LR}} T^{\rm v1v2}_{(2,0)},\ a^{(21)}_{\rm LR} \equiv \langle \tilde{L}_{\rm v_2}(1)|\mathcal{H}^{(1)}_{\rm e-ph}|\tilde{R}_{\rm v_1}(1)\rangle \tag{36}$$

$$T^{\rm v1v2} \xrightarrow{a^{(22)}_{\rm LR}} T^{\rm v1v2}_{(2,0)} \tag{37}$$

$$T^{\rm v2v1} \xrightarrow{-a^{(11)}_{\rm LR}} T^{\rm v1v2}_{(2,0)} \tag{38}$$

$$T^{\rm v2v2} \xrightarrow{-a^{(12)}_{\rm LR}} T^{\rm v1v2}_{(2,0)}\ . \tag{39}$$

In the above equations, the transition amplitudes are expressed via single-particle matrix elements, both diagonal or non-diagonal in the valley index, that involve wave functions from the left and right dot. Notice, that in the dipole approximation these matrix elements are proportional to the corresponding dipole matrix elements: $\langle i|\mathcal{H}^{(1)}_{\rm e-ph}|j\rangle \sim \langle i|\mathbf{r}|j\rangle$. Again, as for the single QD matrix elements, for an ideal interface the non-diagonal in valley matrix elements are exactly zero, see Eqs. (32),(36). For a non-ideal interface these are expected non-zero, and some phonon transitions may be allowed. For the diagonal matrix elements we have the relation: $a^{(22)}_{\rm LR} = a^{(11)}_{\rm LR}$, which is exact for ideal interface. For a non-ideal interface this equality is assumed to hold (at least approximately). Then, from Eqs. (34), (35), (37), (38) it follows that the states $S^{\rm v1v2} - S^{\rm v2v1}$ and $T^{\rm v1v2} + T^{\rm v2v1}$ are protected under phonon emission and therefore blocked. This we call a *spin-valley blockade*. A calculation of the corresponding phonon inelastic decay rates $\Gamma^{(j)}_{\rm in}$ is straightforward, and can be used to construct a set of rate equations describing the transport[6]. Here, however, we will use only the simple relations for the phonon decay amplitudes that leads to the spin-valley blockade, particularly relevant when a finite exchange splitting is accounted.

*Tunneling and exchange splitting.*
To take into account the finite exchange splitting we consider the relevant tunneling Hamiltonians (see, e.g., Ref. 4,10). Neglecting small Coulomb corrections, we calculated for the basis states $S^{\rm v1v1}$, $S^{\rm v1v1}_{(2,0)}$, $T^{\rm v1v1}$:

$$H^{\rm ST}_{\rm v1v1} = \begin{pmatrix} 0 & \sqrt{2}t_c^{(\rm v1)} & 0 \\ \sqrt{2}t_c^{(\rm v1)} & -\varepsilon & 0 \\ 0 & 0 & 0 \end{pmatrix}, \tag{40}$$

and a similarly for the $[\rm v2, v2]$ states, with $\rm v_1 \to v_2$. These Hamiltonians simply reflect the fact that quantum tunneling under a Coulomb barrier does not flip spin (so, the triplet is decoupled), and also conserves the valley

index. A less trivial dynamics is established in the mixed valley subspace. For the singlet basis states $S^{\mathrm{v1v2}}$, $S^{\mathrm{v2v1}}$, $S^{\mathrm{v1v2}}_{(2,0)}$, the tunneling Hamiltonian reads:

$$H^{\mathrm{S}}_{\mathrm{v1v2}} = \begin{pmatrix} 0 & 0 & t_c^{(\mathrm{v2})} \\ 0 & 0 & t_c^{(\mathrm{v1})} \\ t_c^{(\mathrm{v2})} & t_c^{(\mathrm{v1})} & -\varepsilon \end{pmatrix}, \tag{41}$$

and similarly, for the triplet basis states $T^{\mathrm{v1v2}}$, $T^{\mathrm{v2v1}}$, $T^{\mathrm{v1v2}}_{(2,0)}$,

$$H^{\mathrm{T}}_{\mathrm{v1v2}} = \begin{pmatrix} 0 & 0 & t_c^{(\mathrm{v2})} \\ 0 & 0 & -t_c^{(\mathrm{v1})} \\ t_c^{(\mathrm{v2})} & -t_c^{(\mathrm{v2})} & -\varepsilon \end{pmatrix}. \tag{42}$$

The last Hamiltonian is relevant for each spin component of the triplets: $\pm, 0$.

The diagonal in valley tunneling matrix elements in Eqs. (40)-(42) are defined as:

$$t_c^{(\mathrm{vi})} \equiv \langle \tilde{L}_{\mathrm{vi}}(1)|V_L(1)|\tilde{R}_{\mathrm{vi}}(1)\rangle, \quad i = 1, 2, \tag{43}$$

with $V_L(1)$ being the unperturbed confining potential of the left dot. In what follows we take $t_c^{(\mathrm{v1})} = t_c^{(\mathrm{v2})} = t_c$, which is exact for ideal interfaces, and holds (approximately) for non-ideal ones, particularly, since the smooth potential $V_L(1)$ "cannot distinguish valleys".

Here we note that in the above Hamiltonians, Eqs. (40)-(42), we have neglected the interdot intervalley tunneling, $t^{(12)} \equiv \langle \tilde{L}_{\mathrm{v1}}(1)|V_L(1)|\tilde{R}_{\mathrm{v2}}(1)\rangle$, which indeed may be much smaller than the diagonal-in-valley tunneling: $t^{(12)} \ll t_c$, depending on the details of the roughness[5,10]. While $t^{(12)}$ may be of the order of $t_c$ its net effect is mixing of singlet (or triplet) $(1,1)$- and $(2,0)$-states of different valley content[10]. Thus, in addition to the "standard" $(1,1)$-$(2,0)$ anti-crossings at detuning $\varepsilon = 0$, one will get additional $(1,1)$-$(2,0)$ anti-crossings[10] at $\varepsilon = \pm E_V$. This may lift the blockade of certain $(1,1)$-states as they mix with a $(2,0)$-state. For example, the spin-blocked state $T^{\mathrm{v1v2}}$ will mix with $T^{\mathrm{v1v2}}_{(2,0)}$ at $\varepsilon = E_V$. Since, however, the observation of ESR signal made in this paper are at a large range of detunings $\varepsilon$ that are generally different from $E_V$, the analysis of spin-valley blockade and ESR signal are not affected by the presence of non-zero intervalley tunneling, and we dismiss it in the following. A more elaborate account of the effect of intervalley tunneling will be presented elsewhere.

The Hamiltonians, Eqs. (41), (42), provide identical energy spectrum, where the states $|\tilde{2}\rangle = (\mathrm{S}^{\mathrm{v1v2}} - \mathrm{S}^{\mathrm{v2v1}})/\sqrt{2}$ and $|\tilde{4}\rangle = (\mathrm{T}_0^{\mathrm{v1v2}} + \mathrm{T}_0^{\mathrm{v2v1}})/\sqrt{2}$ have energy $E = 0$ independent of dots' detuning $\varepsilon$. Since in the experiment we are in the highly detunned regime, $\varepsilon \gg t_c$, the energies of the states (small admixture of the $(2,0)$ states is neglected) $|\tilde{3}\rangle = (\mathrm{S}^{\mathrm{v1v2}} + \mathrm{S}^{\mathrm{v2v1}})/\sqrt{2}$ and $|\tilde{5}\rangle = (-\mathrm{T}_0^{\mathrm{v1v2}} + \mathrm{T}_0^{\mathrm{v2v1}})/\sqrt{2}$ are approximately shifted by the exchange splitting, $J \simeq 2t_c^2/|\varepsilon|$.

*"Valley parity" conservation.*
Here it is important to note, that $|\tilde{3}\rangle = (\mathrm{S}^{\mathrm{v1v2}} + \mathrm{S}^{\mathrm{v2v1}})/\sqrt{2}$, $|\tilde{5}\rangle = (-\mathrm{T}_0^{\mathrm{v1v2}} + \mathrm{T}_0^{\mathrm{v2v1}})/\sqrt{2}$ are the states that are coupled under quantum tunneling to their $(2,0)$-counterparts, namely the states $S^{\mathrm{v1v2}}_{(2,0)}$ and $T^{\mathrm{v1v2}}_{(2,0)}$, and thus they are correspondingly related via adiabatic change of $\varepsilon$. We can introduce in this respect a new conserved quantity we call a *"valley parity"*. Indeed, under exchange of valley indices, v1 $\leftrightarrow$ v2, the states $|\tilde{3}\rangle$ and $S^{\mathrm{v1v2}}_{(2,0)}$ have positive valley parity, while the state $|\tilde{2}\rangle = (\mathrm{S}^{\mathrm{v1v2}} - \mathrm{S}^{\mathrm{v2v1}})/\sqrt{2}$ related to them via Eq. (41) has opposite (negative) valley parity. Similarly, the states $|\tilde{5}\rangle$ and and $T^{\mathrm{v1v2}}_{(2,0)}$ have a negative valley parity, and the state $|\tilde{4}\rangle = (\mathrm{T}_0^{\mathrm{v1v2}} + \mathrm{T}_0^{\mathrm{v2v1}})/\sqrt{2}$ has opposite (positive) valley parity. Thus, under adiabatic change of $\varepsilon$ the valley parity is conserved, and the relevant states of opposite parity are decoupled. The selection rules we have derived above for the inelastic tunneling (with emission of a phonon) show that the same states $|\tilde{2}\rangle = (\mathrm{S}^{\mathrm{v1v2}} - \mathrm{S}^{\mathrm{v2v1}})/\sqrt{2}$ and $|\tilde{4}\rangle = (\mathrm{T}_0^{\mathrm{v1v2}} + \mathrm{T}_0^{\mathrm{v2v1}})/\sqrt{2}$ that are protected under phonon emission (see also Supplementary Note 4), here are decoupled from their counterparts in the tunneling Hamiltonians, Eqs. (41), (42).

*Finite exchange splitting and multiple anticrossing.*
To take into account the exchange splitting in the mixing Hamiltonians at each anticrossing spot, we rewrite them in the basis of the states $|\tilde{j}\rangle$, dictated by the tunneling $t_c$. For example, for the Hamiltonian of spot I we choose the basis $S^{\mathrm{v1v1}}$, $T_0^{\mathrm{v1v1}}$, $|\tilde{4}_-\rangle$, $|\tilde{5}_-\rangle$

$$H^{\mathrm{I}'} = \begin{pmatrix} J & 0 & i\,b_m & -i\,a_p \\ 0 & 0 & -i\,a_p & i\,b_m \\ -i\,b_m & i\,a_p & X & \delta/2 \\ i\,a_p & -i\,b_m & \delta/2 & X+J \end{pmatrix}, \tag{44}$$

where $a_p \equiv (a_R + b_L)/\sqrt{2}$, $b_m \equiv (a_R - b_L)/\sqrt{2}$. For the spot II the basis is $T_+^{\mathrm{v1v1}}$, $|\tilde{2}\rangle$, $|\tilde{3}\rangle$, $|\tilde{4}\rangle$, $|\tilde{5}\rangle$, and $T_-^{\mathrm{v2v2}}$; so the Hamiltonian is

$$H^{\mathrm{II}'} = \begin{pmatrix} -X & -i\,a_p & -i\,b_m & -i\,a_p & i\,b_m & 0 \\ i\,a_p & 0 & -\delta/2 & 0 & 0 & -i\,a_p \\ i\,b_m & -\delta/2 & J & 0 & 0 & i\,b_m \\ i\,a_p & 0 & 0 & 0 & \delta/2 & -i\,a_p \\ -i\,b_m & 0 & 0 & \delta/2 & J & -i\,b_m \\ 0 & i\,a_p & -i\,b_m & i\,a_p & i\,b_m & X \end{pmatrix} + E_V\,. \tag{45}$$

Finally, for the anticrossing spot III, using the basis $S^{\mathrm{v2v2}}$, $T_0^{\mathrm{v2v2}}$, $|\tilde{4}_+\rangle$, $|\tilde{5}_+\rangle$ we obtain

$$H^{\mathrm{III}'} = \begin{pmatrix} J & 0 & i\,b_m & i\,a_p \\ 0 & 0 & i\,a_p & i\,b_m \\ -i\,b_m & -i\,a_p & -X & \delta/2 \\ -i\,a_p & -i\,b_m & \delta/2 & -X+J \end{pmatrix} + 2E_V\,. \tag{46}$$

Using these Hamiltonians we recalculated the structure of energy levels and the corresponding energy differences capable to reproduce an anticrossing feature in the experimentally observed “bright ESR spot” ($\sim E_V$ at $X \sim 0$). The typical pattern depends on the relative size of the anticrossing splitting and the exchange splitting. For finite $J$ and $J \lesssim |a_R|$ the degeneracy of certain states is lifted (see Fig. 5b of the main text), while the general pattern of the levels and the ESR anticrossing pattern (Fig. 5c) is similar to the case of $J = 0$, as shown in Supplementary Figure 1. For $J \gg |a_R|$, a pattern of multiple anticrossing is formed, Supplementary Figure 3a. By using only the variative AC coupling, we have plotted the combined ESR signal based on all relevant energy differences that forms multiple anticrossing ESR pattern as well, Supplementary Figure 3b. Comparison to an experimentally observed by us multiple anticrossing ESR pattern, Supplementary Figure 3c, suggests that the main role in its description is played by the exchange splitting $J$. This allows us to extract a value of $J \approx 200\,\mathrm{MHz} \approx 0.8\,\mu\mathrm{eV}$ and a value of $t_c \approx 5 - 10\,\mu\mathrm{eV}$ for the interdot detuning $\varepsilon = 50 - 250\,\mu\mathrm{eV}$. An estimation of the tunneling:

$$t_c \simeq \frac{\hbar^2 d}{m_t a_D^3 \sqrt{\pi}} e^{-d^2/a_D^2} \tag{47}$$

(using a biquadratic model of a DQD[4]) is compatible with these values, using a dot radius $a_D \approx 30 - 38\,\mathrm{nm}$ and interdot distance $2d = 110 - 140\,\mathrm{nm}$. Further experimental studies of the multiple anticrossing pattern as well as a complete theoretical description of it will be presented elsewhere.

*Nuclear hyperfine field vs. the exchange splitting.*
Here we describe in more detail a possible explanation of the bright ESR spot, examining also the role of a finite HF magnetic field in Si. Consider again, as an example, the spin-blocked state $T_-^{\mathrm{v1v1}}$. Similar to a GaAs DQD system[7], to lift the blockade a resonant AC microwave field is applied which couples $T_-^{\mathrm{v1v1}}$ to $T_0^{\mathrm{v1v1}}$, Eq. (22). Subsequent lifting of the blockade would happen via the nuclear hyperfine field (HF), bringing the Hamiltonian (see, e.g., Refs. 11,12):

$$\begin{aligned} \hat{H}_{\mathrm{nucl}} = g\mu_B \, [ & (dB_z |S\rangle\langle T_0| + \mathrm{h.c.}) \\ & + \left( \frac{dB_x}{\sqrt{2}} (|S\rangle\langle T_-| - |S\rangle\langle T_+|) + \mathrm{h.c.} \right) \\ & + \left( \frac{dB_y}{\sqrt{2}} (-i|S\rangle\langle T_-| - i|S\rangle\langle T_+|) + \mathrm{h.c.} \right) \\ & + \text{terms} \sim (B_x^a, B_y^a) \\ & + B_z|T_+\rangle\langle T_+| - B_z|T_-\rangle\langle T_-| ] \otimes \mathrm{I}^{\mathrm{v_i v_j}}, \end{aligned} \tag{48}$$

where $B_z = B_z^{(0)} + B_z^a$, and the hyperfine nuclear field in the two dots is combined in the average field and difference: $\mathbf{B}^a \equiv \frac{\mathbf{B}_N^L + \mathbf{B}_N^R}{2}$, $d\mathbf{B} \equiv \frac{\mathbf{B}_N^L - \mathbf{B}_N^R}{2}$. The Hamiltonian $\hat{H}_{\mathrm{nucl}}$ is diagonal in valley index, and couples e.g., $T_0^{\mathrm{v1v1}}$ to the singlet $S^{\mathrm{v1v1}}$, where the last can decay to a $(2,0)$-state. In a GaAs system, typically the exchange splitting is small[7], $J \ll E_N$, and the HF mixing mechanism provides lifting of the blockade (at an AC driving on) for the whole region of Zeeman energies, which is expressed as a sloped straight line on the 2D “frequency-magnetic field” plot (scf. Fig. 3e and Fig. 5a of the main text). However, in our experiment the estimated exchange splitting is a couple of hundred neV,

(see above), and is much larger than the nuclear HF mixing, $J \gg E_N$ (theoretical estimations[13] give $\sigma_N^{\rm Si} \simeq 0.026\,{\rm mT}$ or $E_N = g\mu_B\sigma_N^{\rm Si} \simeq 3\,{\rm neV}$) Thus, out of anticrossing the nuclear HF mixing should be suppressed, since $T_0^{\rm v1v1}$ and $S^{\rm v1v1}$ will be well separated in energy (see Fig. 5b of the main text and Supplementary Figure 3a). As explained above, the ESR signal will become non-zero via the mechanism of spin-valley mixing around the anticrossing point.

For the spin-valley blocked polarized state $T_-^{\rm v1v2} + T_-^{\rm v2v1}$ the story is a bit more involved. An AC driving couples this state *equally* to two states that are degenerate out of anticrossing; namely, these are the states: $|v_{01}\rangle = -|\tilde{2}\rangle + |\tilde{4}\rangle$ and $|m1\rangle = |\tilde{2}\rangle + |\tilde{4}\rangle$. Thus, starting from the polarized state, $\hat{H}_{\rm ac}$, Eq. (21), creates the combination $|v_{01}\rangle + |m1\rangle$, in which the singlet combination $|\tilde{2}\rangle \sim S^{\rm v1v2} - S^{\rm v2v1}$ is canceled, while the triplet $|\tilde{4}\rangle \sim T_0^{\rm v1v2} + T_0^{\rm v2v1}$ is blocked since the nuclear HF coupling to a singlet $[{\rm v}_1, {\rm v}_2]$-state, $S^{\rm v1v2} + S^{\rm v2v1}$ , is again energy suppressed (see Supplementary Figure 3a). At anticrossing the above degeneracy is lifted, as well as the content of the states will change due to the spin-valley mixing described above, and thus the blockade is lifted. This qualitatively explains the "bright ESR spot" at anticrossing.

# Supplementary Note 4
## Spin blockade vs. spin-valley blockade

The type of spin or spin-valley blockade in the case when the AC driving is off was described in full in the main text. Here it is illustrated on Supplementary Figure 4 for the scenario related to our experiment, namely for a relatively large S-T splitting, $\Delta_{\rm ST}^{\rm orb} > 2E_V$. It is important to note, that in our transport experiment all $(1,1)$-states are loaded. On Supplementary Figure 4(a) the dot detuning is $\varepsilon < E_V$. Therefore, the lowest polarized triplet $T_{-}^{\rm v1v1}$ is spin-blocked. In this regime also the state $T_{-}^{\rm v1v2} + T_{-}^{\rm v2v1}$ is spin-valley blocked, due to the selection rules described in Eqs.(37),(38). For the regime of $\varepsilon > E_V$, Supplementary Figure 4(b), the transition $T_{-}^{\rm v1v1} \to T_{(2,0),-}^{\rm v1v2}$ is energetically allowed, however it is still forbidden for an ideal interface, or if the matrix element $a_{\rm LR}^{(21)} \equiv \langle \tilde{L}_{\rm v2}(1)|\hat{H}_{\rm e-ph}|\tilde{R}_{\rm v1}(1)\rangle$, Eq. (36) happens to be small. The transition may be allowed for a non-ideal interface, when the matrix element $a_{\rm LR}^{(21)}$ may become finite. The transport blockade in our experiment, however, cannot discriminate this case, since the state $T_{-}^{\rm v1v2} + T_{-}^{\rm v2v1}$ is still blocked, Supplementary Figure 4(b). That at least one of these blockades should take place is *observed experimentally* as the fact that the transport blockade persists even for $\varepsilon > E_V$. The blockade can be lifted if the transition $T_{-}^{\rm v1v2} + T_{-}^{\rm v2v1} \to T_{(2,0),-}^{\rm v1v1}$ to the first orbital excited state becomes energetically allowed. By inspection, the matrix element, $\langle T_{(2,0)}^{\rm v1v1}|\hat{H}_{\rm e-ph}|T^{\rm v2v1}\rangle = 0$, is zero even for a non-ideal interface, while the other possible (non-diagonal in valley) matrix element may be non-zero:

$$\begin{aligned}\langle T_{(2,0)}^{\rm v1v1}|\hat{H}_{\rm e-ph}|T^{\rm v1v2}\rangle &\simeq -a_{\rm QR}^{(12)} \\ &\equiv -\langle \tilde{Q}_{\rm v_1}^{\rm L}(1)|\hat{H}_{\rm e-ph}^{(1)}|R_{\rm v_2}(1)\rangle\,; \end{aligned} \qquad (49)$$

here $\tilde{Q}_{\rm v_1}^{\rm L}(1)$ is the higher excited orbital state in the left dot, introduced in Supplementary Note 1. Thus, we can reinterpret the measured singlet-triplet splitting

$$\tilde{\varepsilon} \equiv \Delta_{\rm ST}^{\rm exp} = \Delta_{\rm ST}^{\rm orb} - E_V\,, \qquad (50)$$

as is seen on Supplementary Figure 4(b) and commented at length in the main text.

# Supplementary Note 5

## $T_2^*$ and broadening of the ESR line

We consider for simplicity two $(1,1)$-levels, denoted as $T_-$, $T_0$, and couple them via the AC driving, Eq. (22). The state $T_0$ can decay to a $(2,0)$-state either via the nuclear HF coupling, Eq. (48) (as in GaAs), or via the spin-valley mixing described above. We denote this process generically, introducing inelastic decay rate $\Gamma_{\rm in}$. The splitting of the levels $T_-$, $T_0$ is the Zeeman splitting $E_Z = g\mu_B B_z$. In the absence of magnetic field fluctuations the ESR signal is a Lorentzian distribution around the resonance with FWHM of $\Gamma_{\rm in}$: $I(\omega, B_z) = A_0 \frac{\Gamma_{\rm in}/2}{(\hbar\omega - E_Z)^2 + (\Gamma_{\rm in}/2)^2}$, where $A_0$ is an unimportant factor[14]. Given the nuclear HF field fluctuation, $B_z = B_z^{(0)} + B_z^a$, the ESR signal must be averaged over them, where $B_z^a$ is a Gaussian distributed with a standard deviation $\sigma_a = \sigma_{N,z}/\sqrt{2}$ (here, $\sigma_{N,z}$ is the standard deviation of the HF $z$-field distribution in each individual dot). In the case of small inelastic relaxation, $\Gamma_{\rm in} \ll \frac{g\mu_B\sigma_a}{\hbar}$, the Lorentzian is approximated with a $\delta$-function: $\frac{a}{\pi(z^2+a^2)} \to \delta(z)$, and the averaging simply gives:

$$\langle I(\omega, B_z^{(0)})\rangle \propto \frac{1}{\sqrt{2\pi\sigma_a^2}} e^{-\frac{(\hbar\omega - g\mu_B B_z^{(0)})^2}{2\sigma_a^2 (g\mu_B)^2}}, \quad (51)$$

i.e., the form of the ESR line as a function of the external magnetic field, $B_z^{(0)}$, is a Gaussian centered at $\frac{\hbar\omega}{g\mu_B}$. The ESR FWHM is given by:

$$\Delta B_{\rm ESR} = 2\sigma_a\sqrt{2\ln 2} = 2\sigma_{N,z}\sqrt{\ln 2}, \quad (52)$$

allowing us to measure directly the HF field fluctuations in the dot via the measured ESR linewidth. Using this result one can write for the dephasing time of a singlet-triplet qubit[15]:

$$T_{2,ST}^* = \frac{\sqrt{2}\hbar}{g\mu_B\sqrt{\langle \Delta B_{N,z}^2\rangle}} = \frac{\sqrt{2}\hbar}{g\mu_B\sqrt{2}\sigma_{N,z}}$$
$$= \hbar 2\sqrt{\ln 2}/(g\mu_B \Delta B_{\rm ESR}). \quad (53)$$

The narrowest ESR peak we measured has a line width about $\sim 0.15$mT (scf. Fig. 4a of main text), giving a lower bound of the singlet-triplet inhomogeneously broadened spin dephasing time $T_{2,ST}^* \approx 63\,$ns. Indeed, $\sigma_{N,z}$ may be smaller than that extracted from Eq. (52), since the experimentally observed ESR linewidth may be broadened by other mechanisms. One mechanism of broadening may be due to the small exchange splitting $J < |a_R|$ (see Fig. 5b,c of main text, with $J = 0.5|a_R|$), where a bunch of ESR lines are only slightly shifted off each other, and eventually overlap. Another mechanism may be due to the inelastic transition itself, when $\Gamma_{\rm in} \gtrsim \frac{g\mu_B\sigma_a}{\hbar}$.

Assuming the inelastic mechanism only, one has to consider the convolution of the Lorentzian spectrum and the Gaussian distributed HF field. By using the variables $z_0 \equiv \omega - \frac{g\mu_B B_z^{(0)}}{\hbar}$, $\sigma_o \equiv \frac{g\mu_B\sigma_a}{\hbar}$, $a \equiv \frac{\Gamma_{\rm in}}{2}$, and $b_z \equiv \frac{g\mu_B B_z^a}{\hbar}$, the convolution can be represented as a Voigt profile

$$\langle I(\omega, B_z^{(0)})\rangle \propto \int \frac{db_z}{\pi} \frac{a}{(z_0 - b_z)^2 + a^2} e^{-\frac{b_z^2}{2\sigma_o^2}}$$
$$= 2\mathrm{Re}\left[e^{-z^2}\mathrm{erfc}[-iz]\right], \quad (54)$$

where $z \equiv \frac{z_0 + ia}{\sqrt{2}\sigma_o}$ is a complex variable. The FWHM of the Voigt profile is given by the function $f_V = F(f_G, f_L)$ with $f_G = 2\sigma_o\sqrt{2\ln 2}$ and $f_L = 2a = \Gamma_{\rm in}$. A good approximation is $f_V \simeq f_G(\sqrt{1 + 0.2166x^2} + 0.5346x)$, $x \equiv f_L/f_G$. We take into account that $f_G = 2\sqrt{\ln 2}\sigma_{N,z} g\mu_B/\hbar$ and $\sigma_{N,z} \approx 0.016\,$mT in Si[13,16]. For the smallest ESR line width we measured, FWHM $-$ ESR $\simeq 0.15\,$mT, we extract $\Gamma_{\rm in} \simeq 2.6 \times 10^7\, s^{-1}$ and relaxation time $T_1 \simeq 0.0385\,\mu$s that is compatible with the recent measurements of interdot relaxation time $T_1$ in Si/SiO$_2$ DQD structure[17].

# Supplementary References


[1] Yang, C. *et al.* Spin-valley lifetimes in a silicon quantum dot with tunable valley splitting. *Nature Communications* **4**, 2069 (2013).

[2] Tahan, C., Friesen, M. & Joint, R. Decoherence of electron spin qubits in Si-based quantum computers. *Phys. Rev. B* **66**, 035314 (2002).

[3] Burkard, G., Loss, D. & DiVincenzo, D. P. Coupled quantum dots as quantum gates. *Phys. Rev. B* **59**, 2070–2078 (1999).

[4] Culcer, D., Cywiński, L., Li, Q., Hu, X. & Das Sarma, S. Quantum dot spin qubits in silicon: Multivalley physics. *Phys. Rev. B* **82**, 155312 (2010).

[5] Gamble, J. K., Eriksson, M. A., Coppersmith, S. N. & Friesen, M. Disorder-induced valley-orbit hybrid states in Si quantum dots. *Phys. Rev. B* **88**, 035310 (2013).

[6] Ruskov, R. & *et al.* In preparation.

[7] Koppens, F. H. L. *et al.* Driven coherent oscillations of a single electron spin in a quantum dot. *Nature* **442**, 766–771 (2006).

[8] Koppens, F. H. L. *et al.* Detection of single electron spin resonance in a double quantum dot. *J. Appl. Phys.* **101**, 081706 (2007).

[9] Yu, P. & Cardona, M. *Fundamentals of Semiconductors* (Springer, Berlin, 2010).

[10] Culcer, D., Hu, X. & Das Sarma, S. Interface roughness, valley-orbit coupling, and valley manipulation in quantum dots. *Phys. Rev. B* **82**, 205315 (2010).

[11] Jouravlev, O. N. & Nazarov, Y. V. Electron Transport in a Double Quantum Dot Governed by a Nuclear Magnetic Field. *Phys. Rev. Lett.* **96**, 176804 (2006).

[12] Taylor, J. M. *et al.* Relaxation, dephasing, and quantum control of electron spins in double quantum dots. *Phys. Rev. B* **76**, 035315 (2007).

[13] Assali, L. *et al.* Hyperfine interactions in silicon quantum dots. *Phys. Rev. B* **83**, 165301 (2011).

[14] Engel, H.-A. & Loss, D. Detection of Single Spin Decoherence in a Quantum Dot via Charge Currents. *Phys. Rev. Lett.* **86**, 4648–4651 (2001).

[15] Petta, J. R. *et al.* Coherent Manipulation of Coupled Electron Spins in Semiconductor Quantum Dots. *Science* **309**, 2180–2184 (2005).

[16] Maune, B. M. *et al.* Coherent singlet-triplet oscillations in a silicon-based double quantum dot. *Nature* **481**, 344–347 (2012).

[17] Wang, K., Payette, C., Dovzhenko, Y., Deelman, P. W. & Petta, J. R. Charge Relaxation in a Single-Electron Si/SiGe Double Quantum Dot. *Phys. Rev. Lett.* **111**, 046801 (2013).
